# Supplementary material for: FinGPT-HPC: Efficient Pretraining and Finetuning Large Language Models for Financial Applications with High-Performance Computing
Source: arXiv:2402.13533 source file (2024-02-21)
Supplement: Supplementary file 1 [file appendix.tex]

% MNIST\cite{deng2012mnist} is a well-known collection of grayscale images representing handwritten digits. Each image in the dataset is comprised of $28 \times 28$ pixels. The dataset is divided into a training set, containing $60,000$ images, and a testing set, containing $10,000$ images.

% CIFAR-10\cite{krizhevsky2009learning} comprises $60,000$ color images that are categorized into 10 classes, with each image having a size of $32\times 32 \times$ 3. The dataset is divided into $50,000$ training images and $10,000$ testing images, with an even distribution of images among the 10 classes in each set.

% \section*{Results on MNIST and CIFAR-10}

% Both of these datasets are considered lightweight. Typically, when training neural networks on such datasets, the GPU is not fully utilized. 

% In this experiment, we focus on several metrics: accuracy, training time, and speedup.

\section*{Method 3: Decompose-and-fine-tune}

In this method, we have the pretrained model with weight matrix $\bm{W} \in \mathbb{R}^{n \times m}$. We decompose $\bm{W}$ into low-rank matrices, CP and tensor-train layer.
\begin{itemize}
\item For low-rank matrices layer, we use the SVD decomposition to decompose the weight $\bm{W}$. Then we have $\bm{W} \approx \bm{U}\bm{\Sigma} \bm{V}^T$, where $\bm{U} \in \mathbb{R}^{n \times r}, \bm{\Sigma} \in \mathbb{R}^{n \times r}$ and $\bm{V}^T \in \mathbb{R}^{r \times m}$. We get the two low-rank weight matrices $\bm{A} = \bm{U}\Sigma$ and $\bm{B} = \bm{V}^T$, where $\bm{A} \in \mathbb{R}^{n \times r}$ and $\bm{B} \in \mathbb{R}^{r \times m}$.

\item For CP and tensor-train, we organize the weight matrix $\bm{W} \in \mathbb{R}^{n \times m}$ into 4D tensor $\mathcal{W} \in \mathbb{R}^{n_1 \times n_2 \times m_1 \times m_2}$ with $n = n_1 \times n_2$ and $ m = m_1 \times m_2$. Then we decomposition $\mathcal{W}$ into CP or tensor-train layer as in Section \ref{sec:tensor_layer}. 
\end{itemize}

After being decomposed, the model has fewer parameters. We fine-tune the decomposed model to recover its performance.

\section*{The Computation Process of Tensor Cores}
The computation process on tensor cores is as follows:
\begin{itemize}
    %\item Divide $\bm{A}$ into $32$ blocks of size $8 \times 4$, we get blocks $\alpha_{11}, \alpha_{12},...,\alpha_{IJ}$ with $I = 4, J = 8$; Divide $\bm{B}$ into $32$ blocks of size $4 \times 8$, we get blocks $\beta_{11}, \beta_{12},...,\beta_{IJ}$ with $I = 8, J = 4$;
    \item Divide $\bm{A}$ into blocks of size $8 \times 4$, we get $32$ blocks $\bm{\alpha}_{ij}$ with $i = 1,...,4$, $j = 1,...,8$; Divide $\bm{B}$ into blocks of size $4 \times 8$, we get $32$ blocks $\bm{\beta}_{ij}$ with $i = 1,...,8$, $j = 1,...,4$;
    \item Perform matrix multiplication on $\bm{\alpha}_{i1}, \bm{\alpha}_{i2},...,\bm{\alpha}_{i8}$ with $\bm{\beta}_{1j}, \bm{\beta}_{2j},...,\bm{\beta}_{8j}$, respectively, with $i = 1,...,4$, $j = 1,...,4$. These $16$ matrix multiplications can be calculated in parallel using tensor cores. 
    \item For each determined $i$ and $j$, There are $8$ matrices with same size of $8 \times 8$. Add these $8$ matrices, we get the matrix $\bm{\gamma}_{ij}$, which is a block of result matrix $C$. On tensor cores, this process is a part of step-2, without any additional computing overhead.
    \item These $16$ blocks $\bm{\gamma}_{ij}$ with $i = 1,...,4$, $j = 1,...,4$ form the result matrix $\bm{C}$.
\end{itemize}
